# Supplementary material for: SEPAL: Towards a Large-scale Analysis of SEAndroid Policy Customization
Source: arXiv:2102.09764 source file (2021-02-19)
Supplement: Supplementary file 1 [file 9-appendix.tex]

\section*{Appendix} %section 3

\begin{comment}
\subsection{A case for policy format diversity}
\label{subsection:Appendix A}
Table \ref{table:rule diff} shows the different representations of the same rule - granting full permissions to access files labeled by \emph{app\_data\_file} in app processes (except \emph{isolated\_app}).

\begin{table*}[h]
\caption{Different Representations of the Same Rule}
\begin{center}
    \newcommand{\tabincell}[2]{\begin{tabular}{@{}#1@{}}#2\end{tabular}}
    %[!htb] meaning the table is following theparagraph
    \resizebox{\textwidth}{!}{
        \begin{tabular}{llp{15mm}} 
        \hline
        \textbf{File type} & \textbf{Representations of Rules} \\
        \hline
        TE Files & allow \{ appdomain -isolated\_app \} app\_data\_file :file create\_file\_perms \\
        \hline
        CIL File & allow base\_typeattr\_97 app\_data\_file (file (ioctl read write create getattr setattr lock append unlink rename open)) \\
        \hline
        Binary File & \tabincell{l} {allow bluetooth app\_data\_file : file { ioctl read write create getattr setattr lock append map unlink rename open };\\ allow platform\_app app\_data\_file : file { ioctl read write create getattr setattr lock append map unlink rename execute open }; \\allow untrusted\_app app\_data\_file : file { ioctl read write create getattr setattr lock append map unlink rename open }; \\ ......}  \\

        \hline
        \end{tabular}
    }
\label{table:rule diff}        
\end{center}
\end{table*}
\end{comment}

\noindent\textbf{The effectiveness of SEAndroid. }
\label{subsection:effectiveness of SEAndroid}
A robust policy will deny the risky behaviors (access the root directory) performed by unprivileged domains (\emph{untrusted\_app}) even if DAC fails:
\begin{lstlisting}
$ id
uid=0(root) gid=0(root) groups= ... 
context=u:r:untrusted_app:s0:c512,c768
$ ls /
ls: /: Permission denied
$ logcat |grep avc
11-06 06:41:49.193  2810  2810 W ls      :
type=1400 audit(0.0:19): avc: denied { read } for 
name="/" dev="sda43" ino=2 
scontext=u:r:untrusted_app:s0:c512,c768 
tcontext=u:object_r:rootfs:s0 tclass=dir 
permissive=0
\end{lstlisting}
